# Supplementary material for: Plot-guided Adversarial Example Construction for Evaluating Open-domain Story Generation
Source: arXiv:2104.05801 source file (2021-05-25)
Supplement: Supplementary file 1 [file appendix.tex]

\section{Appendices} \label{appendices}

%  In heuristically generated incoherent texts with disjoint and not relevant sequences, PMI of sequence pairs are effective features to distinguish them from coherent texts. 
\begin{table*}
\begin{center}
\small
\begin{tabular}{ll}
\toprule
 \textbf{Metric} & \textbf{Parameters}  \\\midrule
  SENTAVG &  lr=[$2e^{-5}$-$1e^{-3}$], batch\_size=[32-128], epochs=10\\
  Ft\_RoBERTa  &  lr=[$2e^{-5}$-$1e^{-4}$], batch\_size=8, max\_length=128,epochs=3\\
  Ft\_Longformer & lr=[$2e^{-5}$-$1e^{-4}$], batch\_size=3, max\_length=1024,epochs=3\\
  Ft\_GPT2 &  lr=[$2e^{-5}$-$1e^{-4}$], batch\_size=4, max\_length=[128-1024],epochs=3\\
  Ft\_BART & lr=[$2e^{-5}$-$1e^{-4}$], batch\_size=8, max\_length=[128-1024],epochs=3\\
  \bottomrule 
\end{tabular}
\end{center}
\caption{Hyper-parameters used to train models.}
%The words in parentheses shows the aggregation method used to map sentence-level coherency scores to text-level scores.  }
\label{model_param}
\vspace{-1em}
\end{table*}

\subsection{Models Parameters}
We trained both evaluation and language models on a machine with a GeForce RTX 2080 Ti GPU. All pretrained language models have been fine-tuned using AdamW optimizer, while SENTAVG model is optimized using Adam optimizer. In order to replicate results, the hyper-parameters have been shown in Table \ref{model_param}. 
%The maximum run time of training models specified in Table \ref{model_param} on heuristic and adversarial filtered data is less than 4 hours.

\subsection{Human Annotations}
In the conducted AMT experiments, we asked master AMT annotators to evaluate how much do they think the text is plausible. All surveys were repeated if the annotator’s agreement with others was less than 0.2 or the annotator failed the attention check test that was designed to measure its attention. We designed attention-check test as a set of long plausible stories that were ended with signiﬁcantly implausible sentences to make sure annotators rate the text by completely reading each story.

%\subsection{Implausible Constructed Texts}
%In this work, we show that stories generated on the manipulated plots that have injected incoherence sources lead to generate higher-quality implausible samples. Table \ref{man_plt_examples} demonstrates some examples selected from adversarially ﬁltered negative samples generated on manipulated plots. The left column shows the manipulated plots and the right column contains stories generated on those plots.
